# Supplementary material for: Simple linear attention language models balance the recall-throughput tradeoff
Source: arXiv:2402.18668 source file (2025-03-07)
Supplement: Supplementary file 1 [file mamba.tex]

Finally, we show that output in \cref{eq: mamba-ssm} computed by $\Mamba$ is a polynomial in $\vu$ {\em and} ${\exp(\vu)}$.
\begin{proposition}[Recurrent Version]
    Given inputs $\vu, \exp(\vu) \in \R^{\inputLength \times \modelDim}$ with state dimension $\stateDim \in \R$, there exists an equivalent $(\inputLength, \calO(\inputLength\log{\modelDim} + \log^2{\stateDim}), \modelDim, \calO(\modelDim^2 + \stateDim^3), \calO(\modelDim))- \BaseConv$ model that computes the output of the $\Mamba$ layer, cf. \cref{eq: mamba-ssm}. 
\end{proposition}
\begin{proof}
We start by noting that \cref{eq: dep-param-mamba} are all linear functions of the input $\vu$. Thus we can directly obtain $\mB, \mC,$ and $\Delta$ by using $O(1)$-layers of $\BaseConv$ while applying the remembering primitive (\citep[Proposition H.10]{arora2023zoology}). Next, focusing on the time-dependent parameters \eqref{eq: dep-param-mamba}, we first note that each input of $\overline{\mA}$ is given by
\begin{equation}
    \label{eq: entry-Abar}
        \overline{\mA}\brac{i,j} = \exp(\Delta(\vu)\cdot \mA[i,j]).
\end{equation}
Here, $\Delta(\vu)$ is a linear function of the input computed in the previous layer, and since $\overline{\mA}[i,j]$ is taking an exponential of a linear function on the input $\vu$, we can consider it to be pre-computed as the input to the next layer of $\BaseConv$ and treat it as such. Next, we express each entry of $\overline{\mB}$ as a polynomial on $\vu$ and $\exp(\vu)$ as follows:
\begin{equation}
    \label{eq: ssm-param-poly}
        \overline{B}_{i}(\vu, \exp(\vu)) \equiv \sum_{j,k \in [\stateDim] \times [\stateDim]} \mA^{-1}[i,k]\paren{\overline{A}_{k,j}(\vu, \exp(\vu)) - \delta_{k,j}} B_j(\vu).
\end{equation}
For the circuit $\calC^{\overline{B}}_{i}(\vu, \exp(\vu))$ that simulates $\overline{B}_{i}(\vu, \exp(\vu))$, the terms inside the sum can be computed as a multiplication of the input terms in $O(1)$ size and depth, and the sum itself can be computed using $O(\log{\stateDim})$ depth and $O(\stateDim^2)$ size and width. For $\stateDim$ such entries, the resulting circuit then has size and width $O(\stateDim^3)$ with the same depth $O(\log(\stateDim))$. Using \cref{thm: baseconv-ac}, we get $\coyoteTuple{\inputLength}{O(\log^2(\stateDim))}{\modelDim}{O(\stateDim^3)}{\modelDim}$ that computes $\overline{\mB}$.

Moreover, the recurrence for $\vh[i,j]$ in \eqref{eq: ssm-rec} is given by
\[
    \begin{aligned}
        \vh[i,j] &= \overline{\mA}\vh[i-1,j] + \overline{\mB}\vu[i,j] \\
        \vz[i,j] &= \mC\vh[i,j]
    \end{aligned}
 \]
 Since we can compute $\vh[0,j]$ in $\calO(1)$ layers and computing $\overline{\mA}\vh[i,j], \overline{\mB}\vu[i,j]$ and $\mC\vh[i,j]$ needs only $\calO(1)$ layers with each entry from $\vh[i-1,j]$ serving as an input to a multiplication gate along with $\vu[i,j]$, the depth of the circuit is $\calO(\inputLength)$ with width $\modelDim^2$. We can thus apply \cref{thm: gen-ac} to get an $(\inputLength, \calO(\inputLength\log{\modelDim}), \modelDim, \calO(\modelDim^2), \calO(\modelDim))- \BaseConv$ model that can compute $\vh[i,j]$ for each $i \in [\inputLength]$.

Overall, applying \cref{thm: gen-ac} then results in an equivalent $(\inputLength, \calO(\inputLength\log{\modelDim} + \log^2{\stateDim}), \modelDim, \calO(\modelDim^2 + \stateDim^3), \calO(\modelDim))- \BaseConv$ model model.
\end{proof}

\TODO{Review the bounds again.}
\begin{proposition}[Unrolled Version]
    Given inputs $\vu, \exp(\vu) \in \R^{\inputLength \times \modelDim}$ with state dimension $\stateDim \in \R$, there exists an equivalent $(\inputLength, \calO(\log(\inputLength{\modelDim}\stateDim)), \modelDim, \calO(\inputLength\modelDim\stateDim), \calO(\modelDim))-\BaseConv$ model that computes the output of the $\Mamba$ layer, cf. \cref{eq: mamba-ssm}. 
\end{proposition}
\begin{proof}
We start by noting that \cref{eq: dep-param-mamba} are all linear functions of the input $\vu$. Thus we can directly obtain $\mB, \mC,$ and $\Delta$ by using $O(1)$-layers of $\BaseConv$ while applying the remembering primitive (\citep[Proposition H.10]{arora2023zoology}). Next, focusing on the time-dependent parameters \eqref{eq: dep-param-mamba}, we first note that each input of $\overline{\mA}$ is given by
\begin{equation}
    \label{eq: entry-Abar}
        \overline{\mA}\brac{i,j} = \exp(\Delta(\vu)\cdot \mA[i,j]).
\end{equation}
Here, $\Delta(\vu)$ is a linear function of the input computed in the previous layer, and since $\overline{A}_{i,j}$ is taking an exponential of a linear function on the input $\vu$, we can consider it to be pre-computed as the input to the next layer of $\BaseConv$ and treat it as such. Next, we express each entry of $\overline{\mB}$ as a polynomial on $\vu$ and $\exp(\vu)$ as follows:
\begin{equation}
    \label{eq: ssm-param-poly}
        \overline{B}_{i}(\vu, \exp(\vu)) \equiv \sum_{j,k \in [\stateDim] \times [\stateDim]} \mA^{-1}[i,k]\paren{\overline{A}_{k,j}(\vu, \exp(\vu)) - \delta_{k,j}} B_j(\vu).
\end{equation}
For the circuit $\calC^{\overline{B}}_{i}(\vu, \exp(\vu))$ that simulates $\overline{B}_{i}(\vu, \exp(\vu))$, the terms inside the sum can be computed as a multiplication of the input terms in $O(1)$ size and depth, and the sum itself can be computed using $O(\log{\stateDim})$ depth and $O(\stateDim^2)$ size and width. For $\stateDim$ such entries, the resulting circuit then has size and width $O(\stateDim^3)$ with the same depth $O(\log(\stateDim))$. Using \cref{thm: baseconv-ac}, we get $\coyoteTuple{\inputLength}{O(\log^2(\stateDim))}{\modelDim}{O(\stateDim^3)}{\modelDim}$ that computes $\overline{\mB}$.
%\AT{Same as above till here.}

Next, we can unroll the recurrence for $\vh[i,j]$ in \eqref{eq: ssm-rec} as follows:
\begin{equation}
    \label{eq: latent-poly} 
    \vh[i,j,k](\vu, \exp(\vu)) = \sum_{\ell=1}^i \paren{\sum_{k = \ell}^t \paren{\prod_{n \in [i]} \overline{A}_{m,n}(\vu, \exp(\vu))}\overline{B}_{m}(\vu, \exp(\vu)) \cdot \vu[\ell-1, j]} + \overline{B}_{m}(\vu, \exp(\vu)) \cdot \vu[i,j].
\end{equation}
The circuit that simulates the above after taking the outputs of $\calC^{\overline{B}}_{i,j}(\vu, \exp(\vu))$ as input needs to compute the product of the innermost terms which can be done with size and width $O(i)$ and depth $O(1)$. Next, we can compute the inner sum with $O(\log{t})$ depth and $O(t)$ size. Moreover, combined with the outer sum, we need a circuit of size and width $O(t^2)$ and depth $O(\log{t})$. Since $i \le \inputLength$, the circuit $\calC^{h}_{i,j, k}(\vu, \exp(\vu))$ has size and width $O(\inputLength)$ and depth $O(\log{N})$. 

Finally, we can express the output of $\Mamba$ as a polynomial in $\vu$ and $\exp(\vu)$ as
\begin{equation}
    \label{eq: mamba-poly} 
    \vz_{i,j}(\vu, \exp(\vu)) \equiv \sum_{k \in \stateDim} C_k(\vu) \vh[i,j,k](\vu, \exp(\vu)).
\end{equation}
The above can be computed using a circuit of size $O(\stateDim)$ and depth $O(\log{\stateDim})$. Since we need to compute $\inputLength\modelDim$ such output gates, the overall circuit $\vz(\{\vh[i,j,k](\vu, \exp(\vu))\}_{(i,j)})$ has size and width $O(\inputLength\modelDim\stateDim)$ and depth $O(\log{\stateDim})$ depth. 

Overall, composing the above circuits results in a circuit with width $\calO(\stateDim^2 + \inputLength^2 + \inputLength\modelDim\stateDim^2)$ and depth $\calO(\log{\stateDim\inputLength})$. Therefore, applying \cref{thm: baseconv-ac} then results in an equivalent $(\inputLength, \calO(\log(\inputLength{\modelDim}\stateDim)), \modelDim, \calO(\inputLength\modelDim\stateDim), \calO(\modelDim))- \BaseConv$ model.
\end{proof}
